# Supplementary material for: Defining a Metric Space of Host Logs and Operational Use Cases
Source: arXiv:1811.00591 source file (2018-11-01)
Supplement: Supplementary file 1 [file 99-appendix.tex]

\section*{Appendix}
\addcontentsline{toc}{section}{Appendix}
\label{app:appendix}

%% to reference this section use \hyperref[app:appendix]{Appendix}
